# Supplementary material for: SoK: Privacy-Preserving Data Synthesis
Source: arXiv:2307.02106 source file (2023-08-05)
Supplement: Supplementary file 1 [file 4.6_additional.tex]

\subsection{Additional Techniques}
\label{subsec:deep-tech}
\fan{requires work here}
Along a few different dimensions, we introduce the design choices as well as techniques that lead to performance improvement.

\textit{\underline{GAN formulation.}}
The {most common} formulations of GAN include the vanilla GAN~\cite{goodfellow2014explaining,radford2016unsupervised},
% which measures the distribution distance via Jensen-Shannon divergence, 
the Wasserstein GAN~(WGAN)~\cite{arjovsky2017wgan},
% which uses the Wasserstein distance instead, 
and the improved WGAN~\cite{gulrajani2017improved}.
Notably, the theoretical properties of WGAN enables the selection of an optimal clipping threshold for the gradient~\cite{chen2020gs}.
More variants of GAN are summarized in~\Cref{tab:deep}.

\textit{\underline{Privacy accountant.}}
In DP-SGD, the privacy cost accumulates across the training iterations. 
Normally, a privacy accountant is used to track the upper bound of the privacy loss via \textit{adaptive composition} of sequential applications of the Gaussian mechanism.
Research in recent years keep pushing for a tighter bound using different techniques. 
% Proposed by Abadi \etal~\cite{Abadi2016DeepLW} along with the DP-SGD algorithm, the moments accountant derives the bound from the moments.
% The moments accountant~\cite{Abadi2016DeepLW} derives the bound from the moments of the privacy loss.
The moments accountant~\cite{Abadi2016DeepLW} tracks the privacy loss by \textit{adaptive composition} of sequentially applied Gaussian mechanisms and derives the bound of the privacy loss via moments bound.
% , where the moments bound is leveraged to derive an associated upper bound of the privacy loss. 
R\'enyi DP~(RDP)~\cite{mironov2017renyi} builds upon R\'enyi divergence~\cite{renyi1961measures} and supports a tighter privacy analysis;
its appearance boosts the transition to RDP accountant in more recent works~\cite{torkzadehmahani2019dp,chen2020gs,schwabedal2020differentially,kossen2022toward}.

\textit{\underline{Training techniques.}}
GAN is notoriously difficult to train~\cite{salimans2016improved,gulrajani2017improved}.
% DP-SGD further increases the learning instability~\cite{takagi2021p3gm,wang2020dp}, causes additional computational overhead~\cite{xxx}, and leads to performance degradation compared to SGD~\cite{xxx}.
DP-SGD further increases the instability of training~\cite{takagi2021p3gm,wang2020dp}.
Thus, researchers have brought up various techniques %need to be applied 
to facilitate the training procedure. 
% We recall two important steps in DP-SGD: clipping and noise injection. 
To determine a suitable clipping threshold on the gradient norm,
\textit{adaptive clipping} computes a proxy threshold w.r.t. a public dataset~\cite{zhang2018differentially,xu2019ganobfuscator};
\textit{clipping decay} exploits the fact that early stages of training can accommodate more noise~\cite{frigerio2019differentially};
\textit{private norm estimation} obtains the private gradient norms of all samples in a batch and then calculates a DP approximation of their average to use as the clipping norm~\cite{acs2018differentially};
\textit{optimal clipping threshold} can be derived as the approximate upper bound of the gradient norm for certain algorithms~\cite{chen2020gs,zhang2021differentially}.
% dp-GAN~\cite{zhang2018differentially} and GANobfuscator~\cite{xu2019ganobfuscator} propose the adaptive clipping strategy which computes a proxy threshold w.r.t. a public dataset;
% % eliminating the need for a public dataset,
% Frigerio \etal~\cite{frigerio2019differentially} perform clipping decay given that early stages of training can accommodate more noise;
% % much more noise than later stages;
% % a larger amount of noise while less noise can be tolerated in later stages;
% GS-WGAN~\cite{chen2020gs} and Priv-GAN~\cite{zhang2021differentially} derive an approximated upper bound of the gradient norm through the theoretical property of the algorithms.
% of the improved GAN~\cite{gulrajani2017improved}.
% DP-CGAN~\cite{torkzadehmahani2019dp} clip the gradients on real and fake data separately before summing them up and injecting the noise. (i don't understand the benefit of this algorithm)
To decide the scale of the Gaussian noise, 
\textit{noise decay}~\cite{yang2020differential} is proposed  following the similar intuition as that for \textit{clipping decay}.
% Yang \etal~\cite{yang2020differential} propose a noise decay strategy following 
% % the same intuition explained above.
% the aforementioned intuition.
To enable more fine-grained clipping and noise injection, 
stratified clipping is performed over various clustered groups of weights~\cite{zhang2018differentially,wang2020part}.
% parameter grouping is proposed to cluster the weights and perform stratified clipping over different groups~\cite{zhang2018differentially,wang2020part}.
Moreover, %several works find a public dataset helpful in different aspects,
a public dataset is found helpful in several aspects,
\eg, estimating a proxy clipping threshold~\cite{zhang2018differentially,xu2019ganobfuscator} and noise scale~\cite{yu2019differentially},
% serving as a proxy for computing the appropriate clipping threshold~\cite{zhang2018differentially,xu2019ganobfuscator} and noise scale~\cite{yu2019differentially}, 
warm starting~\cite{zhang2018differentially,yang2020differential},
% helping with warm starting~\cite{zhang2018differentially,yang2020differential},
providing a pre-trained embedding model~\cite{fan2021dpnet}.
% The list of techniques could go on and on;
% techniques in both the literature of GAN training and DP-SGD optimization can be leveraged whenever proven helpful.
% techniques from both GAN training (in non-privacy contexts) and DP-SGD optimization (in discriminative modeling) can be borrowed whenever proven helpful.
% ---being the combination of DP-SGD and GAN, 

\textit{\underline{Mixture of models.}} 
% a unique category of models (flexible framework, though the framework itself is questionable)
        Using multiple generative models to model different partitions of the data distribution has been demonstrated to enable easier modeling compared to using one model for all, 
        especially on diverse data samples.
        This further implies benefits on privacy---when fewer training epochs are needed, the accumulated privacy cost will be low.
        In light of such intuition,
        DPGM~\citep{acs2018differentially}, DP-SYN~\citep{abay2018privacy}, and DP-VaeGM~\citep{chen2018differentially}
        use DP-SGD to train DP generative models on disjoint partitions of the dataset, where
        % Their algorithms proceed as follows: first separating the training data into multiple partitions, and then training a DP generative model on each data partition via DP-SGD.
        the partition is performed using either the groundtruth labels~\citep{abay2018privacy,chen2018differentially} or unsupervised clustering through private kernel $k$-means~\citep{acs2018differentially}.
        % can be done via leveraging the groundtruth labels~\citep{abay2018privacy,chen2018differentially} or unsupervised clustering through private kernel $k$-means~\citep{acs2018differentially}.
        % In the partitioning step, the groundtruth labels can be leveraged to guide the partitioning in the supervised setting~\citep{abay2018privacy,chen2018differentially}; or the private kernel $k$-means can be leveraged for an unsupervised clustering~\citep{acs2018differentially}.
        % In the training step, t
        AEs, VAEs, and Restricted Boltzmann Machines~(RBMs)~\cite{tieleman2008training,hinton2012practical} have all been adopted in this framework, but there is no literature that adopts GAN.
        % There is a flexible range of options for the generative models, \eg, AEs~\cite{abay2018privacy}, VAEs~\cite{chen2018differentially}, and Restricted Boltzmann Machines~(RBMs)~\cite{tieleman2008training,hinton2012practical}.
        % There is no literature that fits GAN into this framework, for 
        One 
        potential reason is that GANs are more capable of modeling complicated data distributions.
        % compared to VAEs and RBMs.
        Nevertheless, it is of practical interest to see comparisons between the empirical performance of these different lines of methods.

\textit{\underline{Extension to tabular data.}}\fan{needs work here}
GANs were initially developed for image data~\cite{}.
to extend GANs to deal with tabular data,
it is essential that we embed prior knowledge of the
data (e.g., structural or semantic information) in model
architectures or learning algorithms.
% in the context of privacy, similar requirements and additional challenges.

% Different from image data which GAN is primarily designed for, 
% one unique characteristic of tabular data is the categorical attributes or both categorical and numerical attributes (known as the mixed-type data).
% \mirnegg{Should follow the same notation as in Sec 3: categorical and numerical attribute}. 
% one unique characteristic of tabular data is that it may contain discrete categorical data fields or both discrete and continuous fields (known as the mixed-type data). 
% The presence of 
Discrete categorical data presents a challenge for GAN since the gradient for the discrete variable is zero almost everywhere;
% ---the gradient for the discrete variable is zero almost everywhere, rendering it impossible to train the generator via backpropagation.
even the continuous numerical variable are not the same as those in images due to the lack of Gaussian-like property~\cite{xu2019modeling}.
% To tackle the issue of the discrete data, effective solutions such as the Gumbel softmax~\cite{jang2016categorical} have been proposed; 
To tackle these issues,
% yet for mixed-type data, 
major changes have been made to the data representation, the model architecture, and the learning procedure.

%important table; keep
%\input{tables/tab_GAN_utility_privacy}
